# Supplementary material for: Safety and Liveness Guarantees through Reach-Avoid Reinforcement Learning
Source: arXiv:2112.12288 source file (2021-12-23)
Supplement: Supplementary file 1 [file shielding.tex]

\section{Learning-Based Reach-Avoid Guarantees during Learning and Exploration}
\begin{itemize}
    \item How do we turn this into actual guarantees?
    \item Safe Learning and ``Shielding".
    \item Learned Q-value as an untrusted oracle: check with forward sim.
    \item \textbf{Theorem}: Suppose $\tilde\policy$, simulated forward from $\state$, is predicted to reach $\target$ while avoiding $\failure$. Then, the following least-restrictive ``shielding" law is guaranteed to recursively preserve safety and liveness:
    \begin{equation}
    \policy_{\text{shield}}(\state)=
        \begin{cases}
            \policy_{\text{perf}}(\state)\qquad& \traj^{\tilde\policy}_{\dyn\big(\state,\policy_\text{perf}(\state\big)}(t) \text{ is safe and live}\\
            \tilde\policy(\state)&\text{otherwise}
        \end{cases}
    \end{equation}
    \item Reaching a safe stop or orbit.
\end{itemize}
